# Supplementary material for: Reconstructing occluded Elevation Information in Terrain Maps with Self-supervised Learning
Source: arXiv:2109.07150 source file (2022-01-11)
Supplement: Supplementary file 1 [file S06_appendix.tex]

\section*{APPENDIX}

\subsection{Data Augmentation for Syn2Real}\label{apx:data_augmentation_syn2real}
We use data augmentation on the synthetic dataset to encourage the generalization capabilities of the neural network, tune the distribution of synthetic data to be more similar to the real-world datasets  and thus to minimize the Syn2Real gap. We use the following data augmentation approaches implemented as sequential transformations:
\begin{enumerate}
    \item \textbf{Random vertical scale:} We randomly pick a vertical scaling factor $f_{s,v} \sim \mathcal{U}\left ( 0.8, 10 \right )$. We multiply the elevation of every grid cell in the ground-truth and occluded DEMs with this scaling factor $f_{s,v}$. This helps to generalize to both rather flat and mountainous terrains.
    \item \textbf{Random vertical offset:} Even though we subtract the mean elevation from every elevation value in the DEM to generalize to different elevations from the global navigation coordinate system, we additionally improve generalization by adding a random vertical offset $f_{o,v} \sim \mathcal{U}\left ( \SI{-1}{m}, \SI{1}{m} \right )$ to the synthetic \acp{DEM}.
    \item \textbf{White noise:} We add white noise to the DEM to simulate the signal noise of the depth cameras by sampling elevation noise $w_{w}$ from a normal distribution $w_{w} \sim \mathcal{N}\left ( \SI{0}{m}, \SI{0.001}{m} \right )$ for every grid cell individually.
    \item \textbf{Range adjusted white noise:} The standard deviation of the noise of depth sensors $w_r$ can be modelled as quadratically dependent on the distance of the sensor from the object $d_r$ as $\sigma_{n,r} = f_{n,r} \cdot \left ( \frac{d_r}{d_{r,0}} \right )^2$~\cite{nguyen2012modeling}. We assume planar distances and choose a range normalization factor of $d_{r,0} = \SI{10}{m}$ and a range noise factor $f_{n,r} = \SI{0.01}{m}$. This allows us subsequently to sample the white noise for every grid cell individually as a function of its distance from the robot position: 
    \begin{equation}
        w_r(d_r) \sim \mathcal{N}\left ( 0, \sigma_{n,r}(d_r) \right )
    \end{equation}
    \item \textbf{Gaussian filtered white noise:} When we analysed the real-world datasets recorded with the ANYmal~\cite{hutter2016anymal, hutter2017anymal} robot, we found clusters of noise in the sense that not just a single pixel displayed an offset in elevation compared to the adjacent pixels (e.g.\ white noise) but rather a set of adjacent pixels would display an offset in elevation compared to other pixels in the area (even on completely flat terrain). This motivated us to model a similar noise patterns for the synthetic datasets to bridge the Syn2Real gap more easily. We iterate through all grid cells of a \ac{DEM} and select a grid cell with a probability of \SI{5}{\percent} as the center pixel of a noise cluster. We subsequently sample white noise for the center pixels from the distribution $\bar{w}_{gf,w} \sim \mathcal{N}\left ( \SI{0}{m}, \SI{0.03}{m} \right )$. We finally dilate the noise matrix with a 2D Gaussian filter with standard deviation for the Gaussian kernel $\sigma_{gf,w} = \SI{1}{px}$.
    \begin{equation}
        w_{gf,w} = \frac{1}{2 \pi \sigma_{gf,w}^2} \cdot e^{- \frac{x^2 + y^2}{2 \cdot \sigma_{gf,w}^2}}
    \end{equation}
    \item \textbf{Random occlusion:} Last but not least, we randomly occlude a grid cell with a probability of \SI{2}{\percent} to simulate depredations in the pipeline from depth measurements to the \acp{DEM}~\cite{yao2016iterative, meier2017real}.
% citation for stereo matching failures: \cite{meier2017real}, citation for textureless surfaces: \cite{yao2016iterative}
\end{enumerate}

\subsection{Ray casting}\label{apx:raycasting}
We rely on ray casting to compute occluded \acp{DEM} from the generated ground-truth \acp{DEM} for the synthetic datasets in addition to generating artificial occlusion in the framework of self-supervised learning.
We developed a lightweight C++ component with Python bindings to perform fast ray casting of an entire grid map from a given vantage point\footnote{\url{https://github.com/mstoelzle/grid-map-raycasting}}. The ray casting algorithm (see Algorithm~\ref{algo:raycasting}) takes a grid map (e.g. \ac{DEM}) and a vantage point $\mathbf{x}_v$ in Cartesian coordinates as inputs. The vantage point is specified relative to the center of the \ac{DEM} (e.g. image coordinates $(\frac{u}{2}, \frac{v}{2})$). It iterates with a nested \emph{for} loop through every cell in the grid and subsequently checks whether the cell is visible from the vantage point. This is done by tracing a ray in 3D from the vantage point into direction $\mathbf{d}_{ray}$ of the cell $\mathbf{x}_{gc}$. We initialise the grid cell as not occluded. We step along the ray with a step length of half of the grid resolution $\mathbf{r}_{g} \in \mathbb{R}^{2}$. After each step, we evaluate the current corresponding pixel and extract the elevation of the pixel from the \ac{DEM}. If we have stored an elevation information for the pixel in the \ac{DEM}, we check if the elevation is higher than the current vertical offset of the ray. If that is the case, we break the loop and designate the grid cell, which we are ray casting, as occluded. Otherwise, we continue stepping along the ray until we reach the target grid cell where we break and designate the grid cell as not occluded. We also break when we are past the grid cell by checking if the distance of the vantage point to the current ray position is larger or equal to the distance from the vantage point to the grid cell as we sometimes do not directly reach the grid cell because of numeric inaccuracies.\\

\begin{algorithm}[h]
\SetAlgoLined
\KwResult{$\mathbf{m}_\text{occ}$}
 $u \gets 0$ \;
 $v \gets 0$ \;
 \While{$u < n$}{
    $\mathbf{x}_{gc,x} \gets (-\frac{n}{2} + u)*\mathbf{r}_{g,x}$\;
    \While{$v < m$}{
        $\mathbf{x}_{gc,y} \gets (-\frac{m}{2} + v)*\mathbf{r}_{g,y}$\;
        $\mathbf{x}_{gc,z} \gets \mathbf{m}_{\text{gt}}$\;
    
        \If{$\text{isNan}(\mathbf{m}_{\text{gt}})$}{
            $\mathbf{m}_\mathrm{occ,uv} = True$\;
            \Continue
        }
        
        $\mathbf{d}_\mathrm{ray} \gets \frac{\mathbf{x}_{gc} - \mathbf{x}_{vp}}{\lVert \mathbf{x}_{gc} - \mathbf{x}_{vp} \rVert_2} $\;
        
        occ $\gets$ False\;
        $\mathbf{x}_{rc} \gets \mathbf{x}_{vp}$\;
        \While{occ == False}{
            $\mathbf{x}_{rc} \gets \mathbf{x}_{rc} + 0.5 \cdot \mathbf{d}_{ray} \cdot \min(\mathbf{r}_{g,x}, \mathbf{r}_{g,y})$\;
            
            $u_{rc} \gets round(\frac{n}{2} + \frac{\mathbf{x}_{rc,x}}{\mathbf{r}_{g,x}})$\;
            $v_{rc} \gets round(\frac{m}{2} + \frac{\mathbf{x}_{rc,y}}{\mathbf{r}_{g,y}})$\;
            
            \If{$u == u_{rc}$ and $v == v_{rc}$}{
                \Break
            }
            
            \If{$\lVert \mathbf{x}_{rc} - \mathbf{x}_{vp} \rVert_2 > \lVert \mathbf{x}_{gc} - \mathbf{x}_{vp} \rVert_2$}{
                \Break
            }
            
            \If{isNotNan($\mathbf{m}_{\text{gt},rc}$)}{
                \If{$\mathbf{m}_{\mathrm{gt},rc} > \mathbf{x}_{rc,z}$}{
                    occ $\gets$ True\;
                }
            }
        }
        
        $\mathbf{m}_\mathrm{occ,uv} \gets $ occ\;
        
      $v \gets v + 1$ \;
    }
    $u \gets u + 1$ \;
 }
 \caption{Perform ray casting from vantage point $\mathbf{x}_{vp}$ and with grid resolution $\mathbf{r}_{g}$ for DEM $\mathbf{m}_{\mathrm{gt}}$ and return occluded DEM $\mathbf{m}_\mathrm{occ}$}\label{algo:raycasting}
\end{algorithm}

\subsection{Model architecture}\label{apx:model_architecture visualization}
We adopt an U-Net~\cite{ronneberger2015u} for our neural network architecture as used by many publications in the past few years on the topic of image and video inpainting~\cite{yi2020cosmovae, liu2018image, zhang2018semantic, li2019progressive, chang2019free, wang2020multistage}.
The input is composed of two channels: the occluded elevation map $\mathbf{m}_\mathrm{occ}$ and the binary occlusion mask $\mathbf{M}_\mathrm{occ}$.
As the occluded elevation map contains missing values represented as NaNs for the grid cells which are occluded, we need to replace those NaNs with a floating point number.
We treat this replacement value as a hyperparameter and select $0.0$ after a selection study.
We also implement input and output normalization: we compute the mean of the non-occluded elevation values of a \ac{DEM} and subtract this mean from each elevation value in the grid.
After receiving the output of the model, we add this mean back to each elevation value before computing the loss. 
We adapt our model from the vanilla U-Net~\cite{ronneberger2015u} architecture and make slight adjustments to the number of max-pooling steps because we are dealing with smaller input images (\SI{64x64}{px} instead of \SI{572x572}{px}) than in the original paper~\cite{ronneberger2015u} and we want to keep the network as lightweight as possible.
Thus, we limit the number of max-pooling operations to 3 (instead of 5 in the original paper) and treat the number of channels in each hidden dimension as a hyperparameter for which we select 64, 128, and 256 channels for our hidden dimensions. 
Analogue to the original paper~\cite{ronneberger2015u}, we use double convolutions with kernel 3 and padding 1 at every hidden dimension for the contracting path. Every convolution is followed by 2D batch norm and a \ac{ReLU}. 
After the encoder, we directly enter the expansive path without a latent space. 
Bilinear up-sampling with a scale factor of two is used for every decoding step with subsequent concatenation with the skip connection data. 
Analogue to the encoder, every double convolution is followed by a 2D batch norm and a \ac{ReLU}. 
Ablation study experiments showed that skip connections are absolutely essential for decent reconstruction performance. 
We visualize the adapted U-Net architecture in Figure~\ref{fig:unet}.

\begin{figure}[h]
  \centering
  \includegraphics[width=1\columnwidth]{figures/unet.pdf}
  \caption{U-Net~\cite{ronneberger2015u} as implemented in this work. We input the occluded DEM $\mathbf{m}_\mathrm{occ}$ and a binary occlusion mask $\mathbf{M}_\mathrm{occ}$ and output the reconstructed DEM. $\mathbf{m}_\mathrm{rec}$}\label{fig:unet}
\end{figure}
